# Supplementary material for: Reclaiming Low-Quality Instruction Data with Rule-Guided LLM Reconstruction
Source: arXiv:2510.23160 source file (2026-10-14)
Supplement: Supplementary file 1 [file H_LLM_Role.tex]

\paragraph{Use of Large Language Models} In our \method, the LLM is designed as an atomic capability and primarily contributes to the data quality evaluation and data fusion stages.
