# Supplementary material for: Reclaiming Low-Quality Instruction Data with Rule-Guided LLM Reconstruction
Source: arXiv:2510.23160 source file (2026-10-14)
Supplement: Supplementary file 2 [file more_experiment.tex]

% \paragraph{Baselines} The full synthetic dataset generated by \method consists of 54888 samples drawn from the LQ Set (123786 samples): 15488 samples are obtained via intra-cluster fusion, and 39400 via inter-cluster fusion. To assess the effectiveness of \method, we adopte 13 representative data‑selection methods as baselines, applying each to the LQ Set for fair comparison: \circled{1} {\large\textit{Vanilla Base Model}} denotes the original base model without any fine-tuning; \circled{2} {\large\textit{LQ Set \& HQ Set}} represent the low-quality set (123786 samples) and high-quality set (131247 samples), both extracted from {\large\textit{Full Set}}. We first employ the LLM‑rating step from $\mathrm{DS}^{2}$~\cite{pang2024improving} to assign overall‑quality scores to every sample in the source data pool. Subsequently, we apply the clusterability-based method~\cite{zhu2021clusterability} to correct the potential scoring bias. Samples with curated scores in the range [0, 2] form the LQ Set, while those with scores in [3, 5] compose the HQ Set; \circled{3} {\large\textit{Full Set}} comprises 300932 samples as our source data pool; \circled{4} {\large\textit{Completion Length}} utilizes the length of the whole corpus as an indicator to assess to sample quality. Intuitively, longer completions tend to reflect richer, higher-quality dialogues, providing more context, depth, and informativeness; \circled{5} {\large\textit{$\mathrm{KNN}_{i}$}} is defined as the Average Euclidean Distance (AED) from each raw embedding vector to its $i$ nearest neighbors within the embedding space. We obtain all embeddings using the same model\footnotemark[\getrefnumber{fn:BAAI/bge-large-en huggingface.co/BAAI/bge-large-en-v1.5}] and then rank samples by their AED in ascending order. Samples with smaller distances are considered more centrally located and thus more representative in the embedding space; \circled{6} {\large\textit{Perplexity}}, computed using a pre-trained language model in a zero‑shot fashion, is employed as the evaluation metric. We compute perplexity for each sample using LLaMA‑3.1‑8B‑Instruct model. Samples are then selected in descending order of perplexity. A larger perplexity score indicates greater model uncertainty, suggesting the sample is more difficult or rare; \circled{7} {\large\textit{Random Selection}}, all samples are randomly selected; \circled{8} {\large\textit{AlpaGasus (Random)}}~\cite{chen2023alpagasus} employs ChatGPT to score each sample and retains only the highest-rated samples for fine-tuning. For a fair comparison, we use gpt-4o-mini\footnotemark[\getrefnumber{fn:gpt-4o-mini-2024-07-18}] as the scoring model. Since the number of samples receiving the top score (55530) exceeds our required dataset size (54888), we randomly sample the final set from among those highest-scoring samples; \circled{9} {\large\textit{IFD}}~\cite{li-etal-2024-quantity}, Instruction‑Following Difficulty, quantifies how much an instruction aids a model’s generation by comparing the model’s loss (or perplexity) with and without instruction context. A higher IFD score indicates that the model is less familiar with a given sample, implying this sample is relatively rare; \circled{10} {\large\textit{Superfiltering}}~\cite{li2024superfiltering} utilizes a small and weaker model, GPT-2~\cite{radford2019language}\footnote{Hugging Face Model: openai-community/gpt2\label{fn:gpt2}}, for the data selection; \circled{11} {\large\textit{DEITA}}~\cite{liu2024makesgooddataalignment} jointly uses two pre-trained scoring model to rate data samples based on complexity\footnote{Hugging Face Model: hkust-nlp/deita-complexity-scorer\label{fn:deita-complexity-scorer}} and quality\footnote{Hugging Face Model: hkust-nlp/deita-quality-scorer\label{fn:deita-quality-scorer}}. However, all the single-turn samples are rated as 3. In order to further demonstrate the effectiveness of this method, we also employ our curated scores as an alternative, which is reported as {\large\textit{DEITA (Our Curated Score)}}; \circled{12} {\large\textit{RDS+}}~\cite{ivison2025large}, representation-based data selection, utilizes a weighted mean pooling of a pre-trained model’s final hidden states for computing the cosine similarity between the raw dataset and the validation set. Accordingly, this method extracts an optimal subset from the source pool for each test benchmark individually. Nevertheless, this test-specific subset does not necessarily yield superior performance on that specific benchmark, in fact, a subset curated using a different validation set may outperform it. Consequently, to showcase the upper performance bound of this method, we also report the best result achieved for each test benchmark, denoted as {\large\textit{RDS+ (best)}}; \circled{13} {\large\textit{$\mathrm{DS}^{2}$}}~\cite{pang2024improving} leverages LLM-generated quality scores, corrected via a score transition matrix, and further integrates cosine similarity-based long-tail scoring to select samples that are both high-rated and rare.
