# Supplementary material for: Reclaiming Low-Quality Instruction Data with Rule-Guided LLM Reconstruction
Source: arXiv:2510.23160 source file (2026-10-14)
Supplement: Supplementary file 3 [file other_preliminary.tex]

\subsection{Average Silhouette Score}
% \vspace{-0.4cm}
Clustering quality hinges on both how tightly points group within their own clusters (cohesion) and how well they separate from other clusters (separation). The Silhouette Score uniquely captures both dimensions in a single metric, enabling an immediate, interpretable gauge of cluster validity~\cite{rousseeuw1987silhouettes}. Mathematically, for each data point $i$ 
% \wjh{not define data point as $i$, which is often denoted as index. We can use maybe $x_i$ or some other choices}
assigned to cluster $C_{I}$, the cohesion $a(i)$ and separation $b(i)$ are defined as follows:
\begin{align}\label{formula_cohesion_seperation}
a(i) = \frac{1}{|C_{I}|-1}\sum_{\substack{j\in C_{I}, j\neq i}}d(i,j),\quad
b(i) = \min_{J\neq I}\frac{1}{|C_J|}\sum_{j\in C_J}d(i,j), \tag{1}
\end{align}
where $d(\cdot,\cdot)$ represents the Euclidean distance; $a(i)$ is computed as the average distance between point $i$ and all other members of its own cluster; $b(i)$ denotes the minimum of the average distances from $i$ to the members of any other cluster $C_J$. Based on these quantities, the silhouette coefficient $s(i)$ for each point $i$ is then defined as:
\begin{align}\label{formula_silhouette}
s(i) = \frac{b(i)-a(i)}{\max\{a(i),b(i)\}},\quad -1 \le s(i) \le 1, \tag{2}
\end{align}
where $\max\{a(i),b(i)\}$, normalizing denominator, ensures $s(i)$ lies in the range of [-1,1]. When $s(i)\approx +1$, the intra-cluster distance $a(i)$ is much smaller than the nearest inter-cluster distance $b(i)$, indicating that point $i$ lies deep inside its own cluster and is well separated from all others. When $s(i)\approx 0$, the cohesion and separation distances are approximately equal ($a(i)\approx b(i)$), suggesting that $i$ sits near the boundary between two clusters and could plausibly belong to either. Conversely, when $s(i)\approx -1$, the intra-cluster distance exceeds the nearest inter-cluster distance ($a(i)>b(i)$), which implies that $i$ is likely misassigned and would be better placed in its neighboring cluster. Finally, the overall clustering quality is captured by the Average Silhouette Score $\tilde s$, defined as the mean of all individual silhouette coefficients $s(i)$:
\begin{align}\label{formula_avg_silhouette_score}
\tilde s = \frac{1}{N}\sum\nolimits_{i=1}^{N} s(i), \tag{3}
\end{align}
where $N$ is the total number of examples. A higher $\tilde s$ (closer to +1) indicates that clusters are both cohesive, whereas values near 0 or negative signal ambiguous or poor clustering assignments.
% Mathematical Symbol Representation For Formula \ref{formula_silhouette}:
% \begin{enumerate}
% \item $\tilde s(k)$: \emph{average Silhouette Score} for a k-cluster solution, computed by averaging all individual sample coefficients; quantifies overall cluster quality, with higher values indicating more cohesive and well‑separated clusters
% \item $n$: total number of corpora
% \item $s(i)$: \emph{Silhouette Coefficient} of the $i^{th}$ corpus, within the range [-1, 1], measuring how well the $i^{th}$ corpus fits its assigned cluster versus its nearest alternative
% \item $a(i)$: \emph{intra‑cluster distance} for the $i^{th}$ corpus, the average distance from the $i^{th}$ corpus to all other corpora in its own cluster, $|C_{\ell_i}|$, indicating cluster cohesion
% \item $|C_{\ell_i}|-1$: number of other samples in the cluster of the $i^{th}$ corpus
% \item $b(i)$: the \emph{nearest‑cluster distance}, the minimum, over all clusters $j \neq \ell_i$, of the average distance from the $i^{th}$ corpus to every corpus in cluster $C_j$, capturing the closest alternative grouping
% \end{enumerate}
% \vspace{-0.5cm}
